# Supplementary material for: Onset of glassiness in two-dimensional ring polymers: interplay of stiffness and crowding
Source: arXiv:2306.02403 ancillary file (2023-06-04)
Supplement: Supplementary file 1 [file Supplementary.pdf]

**Supplementary Information:**

# Onset of glassiness in two-dimensional ring polymers: interplay of stiffness and crowding

Sayantan Ghosh,[1,2,a] Satyavani Vemparala,[1,2,b] and Pinaki Chaudhuri[1,2,c]

[1] *The Institute of Mathematical Sciences, C.I.T. Campus, Taramani, Chennai 600113, India*

[2] *Homi Bhabha National Institute, Training School Complex, Anushakti Nagar, Mumbai, 400094, India*

(Dated: 30 May 2023)

[a] Electronic mail: sayantang@imsc.res.in

[b] Electronic mail: vani@imsc.res.in

[c] Electronic mail: pinakic@imsc.res.in

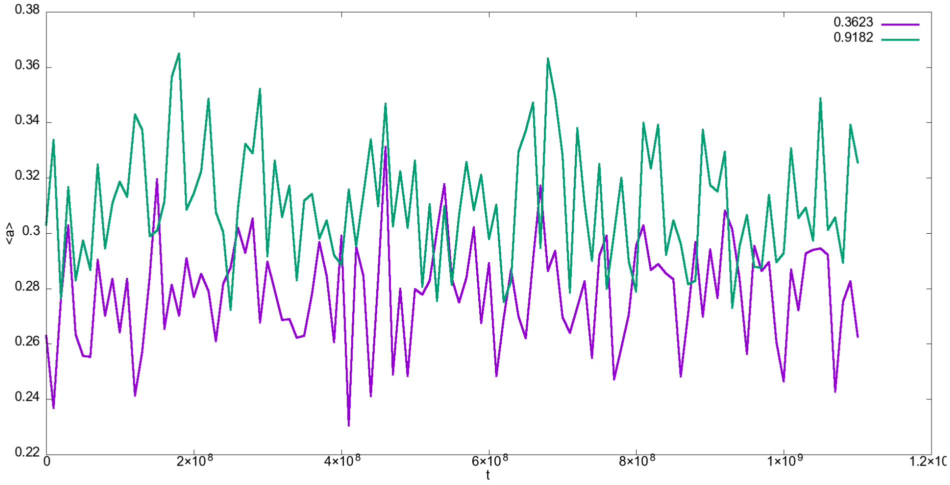


FIG. S.1. $K_\theta = 1$. Time series of asphericity, averaged over all rings within one configuration, at densities 0.3623 and 0.9182.

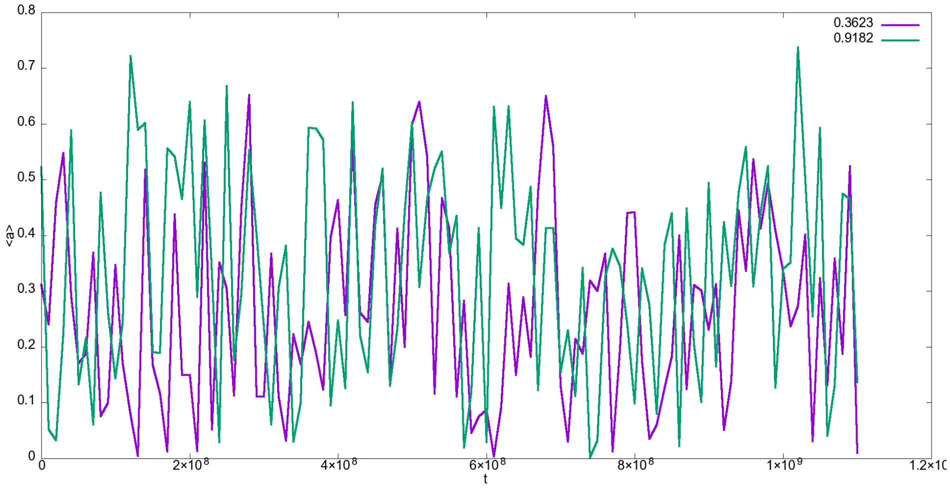


FIG. S.2. $K_\theta = 1$. Time series of asphericity of selected individual rings, at densities at densities 0.3623 and 0.9182.

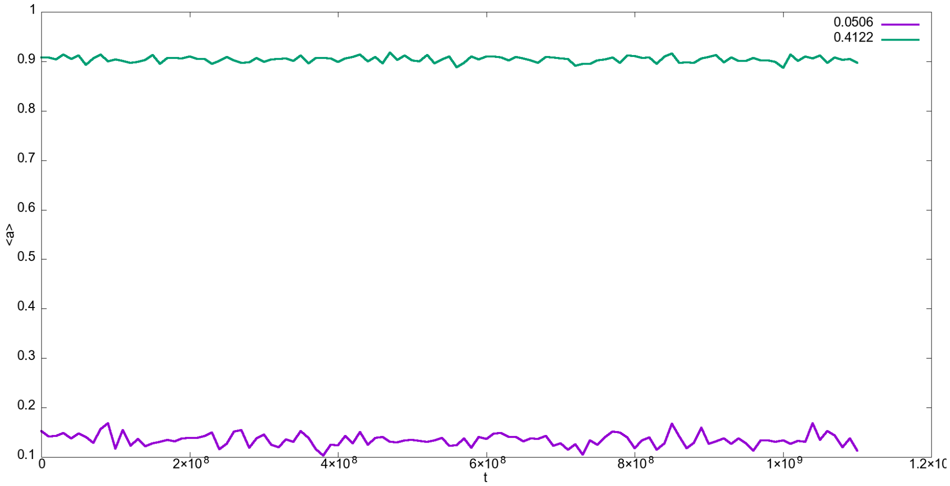


FIG. S.3. $K_\theta = 20$. Time series of asphericity, averaged over all rings within one configuration, at densities 0.0506 and 0.4122

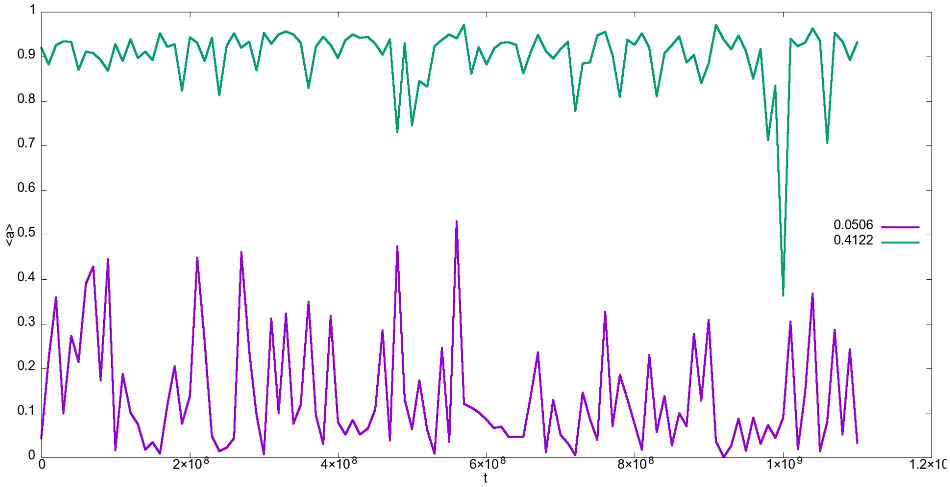


FIG. S.4. $K_\theta = 20$. Time series of asphericity of selected individual rings, at densities 0.0506 and 0.4122.
